# Supplementary material for: Scalar and Vector Airborne Platform Calibration Using Quantum and Classical Magnetometers and Inertial Sensors
Source: arXiv:2605.04951 source file (2026-05-06)
Supplement: Supplementary file 1 [file appendices.tex]

\section{}
\label{app:induced}
The induced coefficient term $B^p_{ind}$ in the scalar \ac{TL}-approximation can be rewritten to:
\begin{equation}
\begin{split}
    B^p_{ind} &=  \bfN  \bfB_e^b \cdot \hbfB_e^b = \begin{pmatrix}
    \beta_1 & \beta_2 & \beta_3 \\ \beta_4 & \beta_5 & \beta_6 \\ \beta_7 & \beta_8 & \beta_9 \end{pmatrix}  \bfB_e^b \cdot \hbfB_e^b \\
    &= \dfrac{1}{\left \lVert\bfB_e\right \rVert}\begin{pmatrix}
    \beta_1 B_x + \beta_2 B_y + \beta_3 B_z \\ \beta_4 B_x + \beta_5 B_y + \beta_6 B_z\\ \beta_7 B_x + \beta_8 B_y + \beta_9 B_z \end{pmatrix} \cdot \begin{pmatrix}
    B_x  \\ B_y \\  B_z \end{pmatrix} \\
    % USE \bigg HERE INSTEAD OF \left
    &= \dfrac{1}{\left \lVert\bfB_e\right \rVert} \biggl( \beta_1 B_x^2 + \beta_2 B_y B_x + \beta_3 B_z B_x + \beta_4 B_xB_y \\
    &\quad + \beta_5 B_y^2 + \beta_6 B_z B_y + \beta_7 B_x B_z + \beta_8 B_y B_z + \beta_9 B_z^2 \biggr)  \\
    &= \dfrac{1}{\left \lVert\bfB_e\right \rVert} \biggl( \beta_1 B_x^2 + (\beta_2 + \beta_4) B_x B_y + (\beta_3 + \beta_7) B_x B_z \\
    &\quad + \beta_5 B_y^2 + (\beta_6+\beta_8) B_y B_z + \beta_9 B_z^2\biggr) \\
    &=\begin{pmatrix}
    \beta_1 & (\beta_2 + \beta_4) & (\beta_3 + \beta_7) \\ 0 & \beta_5 & (\beta_6 + \beta_8) \\  0 & 0 & \beta_9 \end{pmatrix}  \bfB_e^b \cdot \hbfB_e^b.
\end{split}
\label{eq:B_p_ind}
\end{equation}
By defining $b_1 = \beta_1 $, $b_2 = \beta_2 + \beta_4 $, $b_3 = \beta_3 + \beta_7 $, $b_4 = \beta_5$,  $b_5 = \beta_6 + \beta_8$, $b_6 = \beta_9$, we end at
\begin{equation}
    B^p_{ind} =  \begin{pmatrix}
    b_1 & b_2 & b_3 \\ 0 & b_4 & b_5 \\ 0 & 0 & b_6
    \end{pmatrix}  \bfB_e^b \cdot \hbfB_e^b.
\end{equation}

% you can choose not to have a title for an appendix
% if you want by leaving the argument blank
%\section{}
%Appendix two text goes here.
